# Supplementary material for: hp3D User Manual
Source: arXiv:2207.12211 source file (2023-09-21)
Supplement: Supplementary file 1 [file comments.tex]

\section*{Historical Comments}
